# Supplementary material for: Bayesian non-parametric ordinal regression under a monotonicity constraint
Source: arXiv:2007.01390 ancillary file (2022-02-11)
Supplement: Supplementary file 1 [file Ordinal_monotonic_regression_Supplement.pdf]

# Supplementary Material for Non-parametric ordinal regression under a monotonicity constraint

Olli Saarela<sup>\*1</sup>, Christian Rohrbeck<sup>2</sup>, and Elja Arjas<sup>3,4</sup>

<sup>1</sup>Dalla Lana School of Public Health, University of Toronto

<sup>2</sup>Department of Mathematical Sciences, University of Bath

<sup>3</sup>University of Helsinki

<sup>4</sup>University of Oslo

July 2, 2020

## **Abstract**

This Supplementary Material provides additional results for the simulation and case studies in Section 3 and Section 4 of the main paper.

---

<sup>\*</sup>Correspondence to: Olli Saarela, Dalla Lana School of Public Health, 155 College Street, Toronto, Ontario M5T 3M7, Canada. Email: [olli.saarela@utoronto.ca](mailto:olli.saarela@utoronto.ca)

## S1 Supplementary Material for Section 3.1

### S1.1 Formulas for the survival functions

The formulas for the considered sets of survival functions  $S(1 \mid \mathbf{x}), \dots, S(5 \mid \mathbf{x})$  in Section 3.1 are provided in the following.

#### Linear

$$S(k \mid \mathbf{x}) = a_k + b_k x_1 + c_k x_2$$

with values

|       | $S(1 \mid \mathbf{x})$ | $S(2 \mid \mathbf{x})$ | $S(3 \mid \mathbf{x})$ | $S(4 \mid \mathbf{x})$ | $S(5 \mid \mathbf{x})$ |
|-------|------------------------|------------------------|------------------------|------------------------|------------------------|
| $a_k$ | 1.0                    | 0.6                    | 0.4                    | 0.2                    | 0.0                    |
| $b_k$ | 0.0                    | 0.2                    | 0.15                   | 0.15                   | 0.2                    |
| $c_k$ | 0.0                    | 0.2                    | 0.15                   | 0.15                   | 0.2                    |

#### Continuous

$$S(k \mid \mathbf{x}) = \begin{cases} a_k & \text{if } (1 - x_1)^2 + (1 - x_2)^2 > 1 \\ a_k + b_k [1 - (1 - x_1)^2 + (1 - x_2)^2] & \text{if } (1 - x_1)^2 + (1 - x_2)^2 \leq 1 \end{cases}$$

with values

|       | $S(1 \mid \mathbf{x})$ | $S(2 \mid \mathbf{x})$ | $S(3 \mid \mathbf{x})$ | $S(4 \mid \mathbf{x})$ | $S(5 \mid \mathbf{x})$ |
|-------|------------------------|------------------------|------------------------|------------------------|------------------------|
| $a_k$ | 1.0                    | 0.6                    | 0.5                    | 0.4                    | 0.3                    |
| $b_k$ | 0.0                    | 0.4                    | 0.3                    | 0.2                    | 0.1                    |

#### Discontinuous

$$S(k \mid \mathbf{x}) = \log(a_k + b_k x_1 + c_k x_2 + 0.3 \times \mathbb{1}\{\max(x_1, x_2) > u_k\})$$

with values

|       | $S(1 \mid \mathbf{x})$ | $S(2 \mid \mathbf{x})$ | $S(3 \mid \mathbf{x})$ | $S(4 \mid \mathbf{x})$ | $S(5 \mid \mathbf{x})$ |
|-------|------------------------|------------------------|------------------------|------------------------|------------------------|
| $a_k$ | $e$                    | 1.7                    | 1.4                    | 1.25                   | 1.1                    |
| $b_k$ | 0.0                    | 0.2                    | 0.15                   | 0.15                   | 0.0                    |
| $c_k$ | 0.0                    | 0.4                    | 0.4                    | 0.3                    | 0.25                   |
| $u_k$ | 1.0                    | 0.4                    | 0.5                    | 0.6                    | 0.7                    |

## S1.2 Trace plots

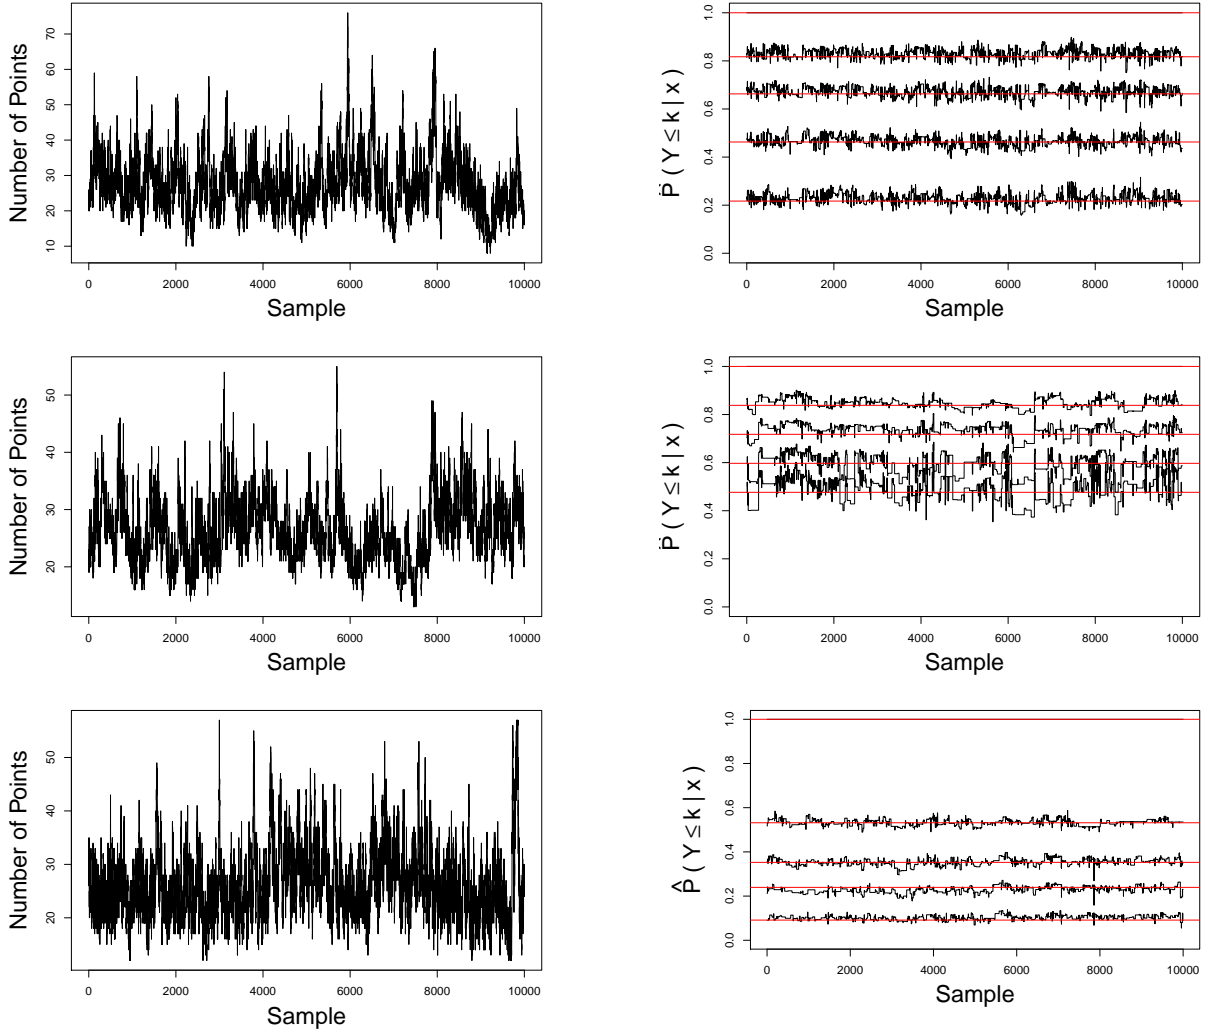

Figure S1: Trace plots for the number of marked points (left) and  $\lambda_1(\mathbf{x}), \dots, \lambda_5(\mathbf{x})$  for an observed data point (right). From top to bottom, the rows correspond to the linear, continuous and discontinuous function sets. The red lines in the right plots illustrate the true function values.

## S1.3 Function estimates

The posterior mean estimates in Figure 2 of the main paper indicate that our methodology correctly identifies the structure of the underlying model functions. The plots in Figure S2 further show that the true function almost always lies within the estimated central 90% credible interval.

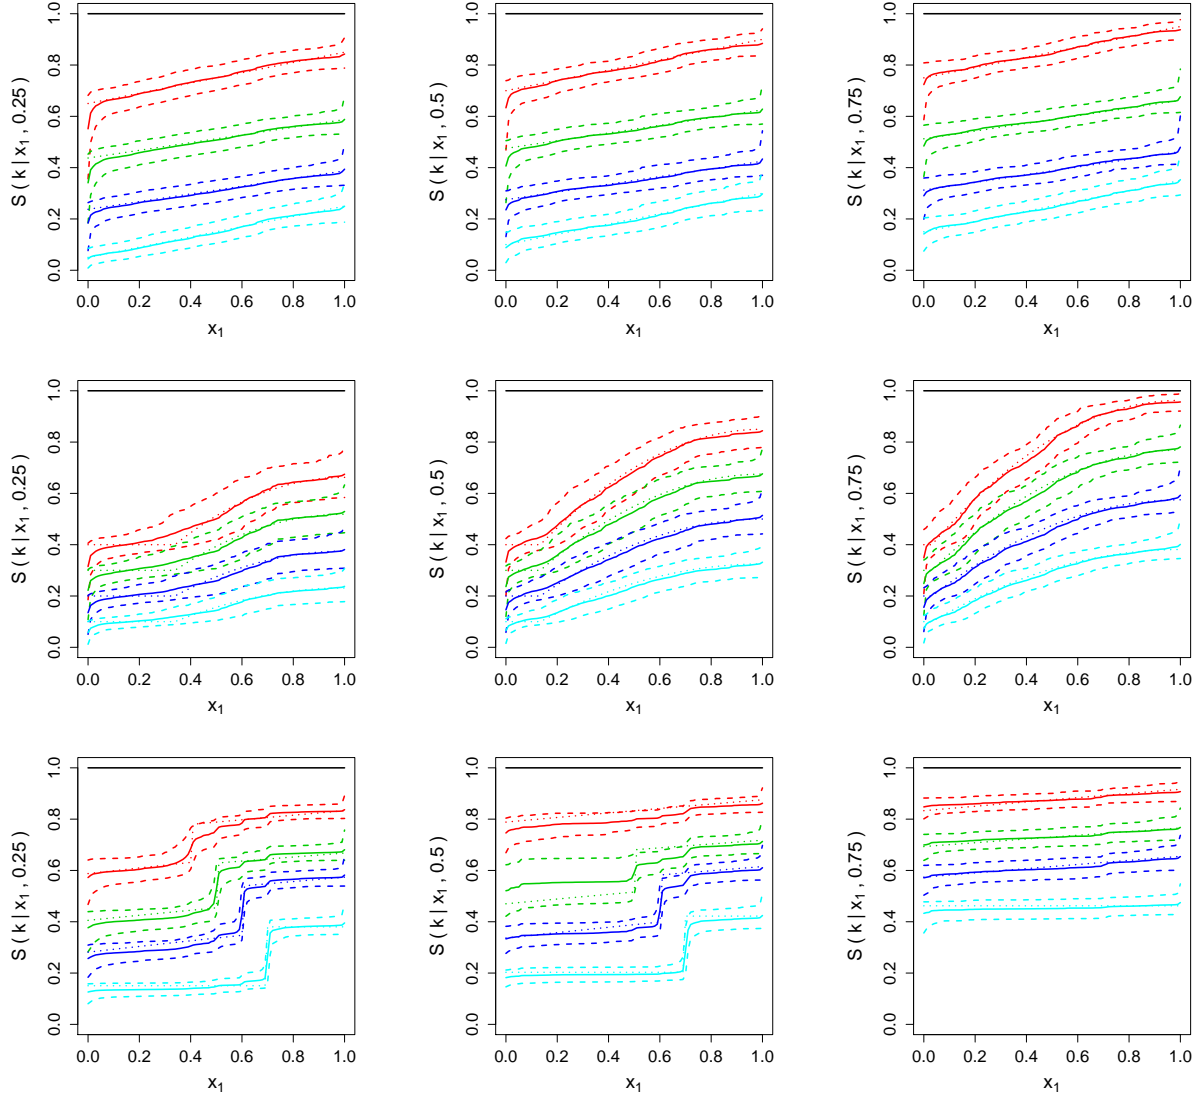

Figure S2: Posterior mean estimates (solid) and central 90% credible intervals (dashed) for  $\lambda_k(x_1, 0.25)$ ,  $\lambda_k(x_1, 0.5)$  and  $\lambda_k(x_1, 0.75)$  (left to right),  $k = 1, \dots, 5$ , averaged over 20 repetitions with  $N = 5,000$  data points for the three considered function sets. The dotted lines illustrate the true functions. From top to bottom, the rows refer to the linear, continuous and discontinuous function sets.

#### S1.4 Comparison of uniform and conditional beta prior

In Sections 2.3.2 and 3.1, we highlighted that monotonic regression estimates tend to be inconsistent at the boundaries of the support of the data. This issue is visible in Figure S3, which shows that for the set of linear survival functions, the highest estimation errors usually occur close to the boundaries, in particular, close to the origin. Similar effects are found for the other function sets. We thus proposed an alternative prior in Section 2.3.2 to reduce this

'spiking problem'. Figure S4 indicates that this change of the prior, with the user-specified prior parameter  $d$  set to  $d = K = 5$ , indeed has the desired effect, without otherwise significantly changing the overall function estimates.

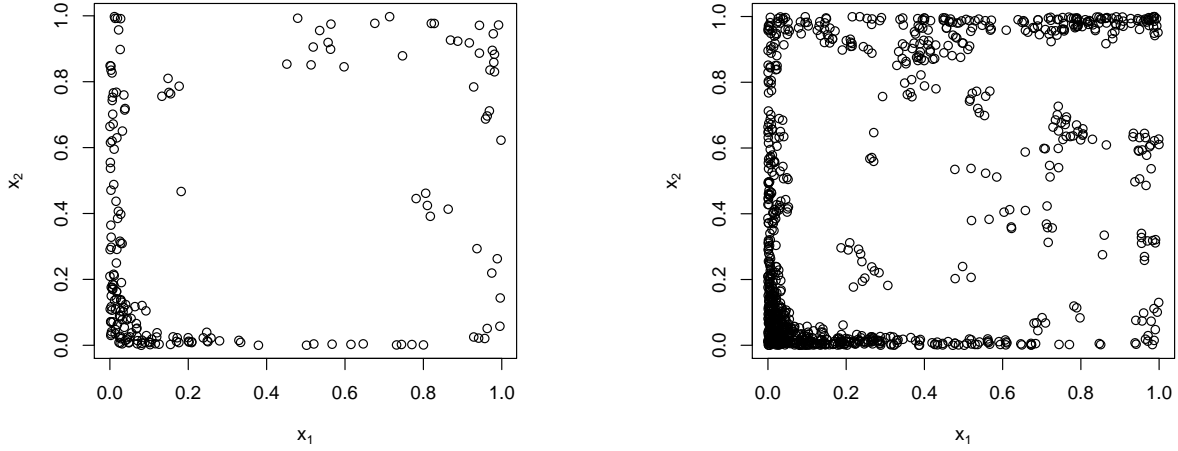

Figure S3: Covariate values with  $|\hat{p}(Y = y_n | \mathbf{x}_n) - \mathbb{P}(Y = y_n | \mathbf{x}_n)|$  exceeding the 99% quantile of the absolute difference for the data sets with  $N = 1000$  (left) and  $N = 5000$  (right) data points for the set of linear survival functions.

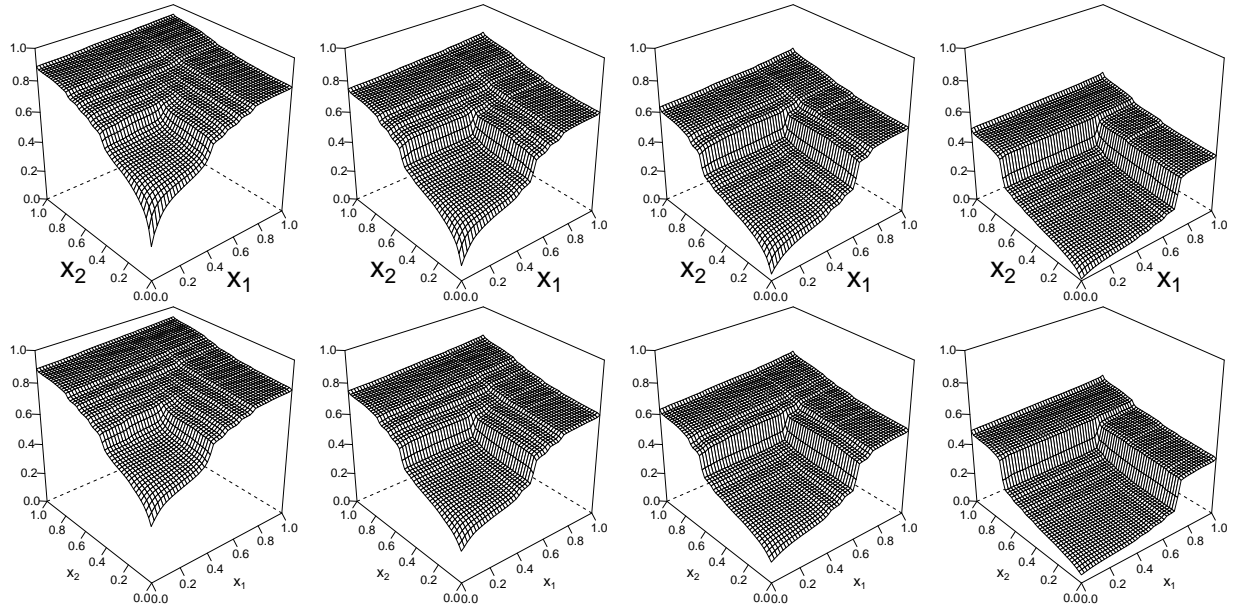

Figure S4: Posterior mean estimates based on the uniform (top) and conditional beta (bottom) priors for  $\lambda_2$ ,  $\lambda_3$ ,  $\lambda_4$  and  $\lambda_5$  (left to right) for the discontinuous functions set. The estimates are averaged across the 20 repetitions with  $N = 5,000$  data points.

## S2 Supplementary Material for Section 3.2

### S2.1 Underlying functions

The functions  $\lambda_2, \dots, \lambda_5$  are defined as  $\lambda_k(\mathbf{x}) = -2 + 4S^*(k \mid \mathbf{x})$ ,  $k = 2, \dots, 5$ , where  $S^*(k \mid \mathbf{x})$  corresponds to the survival function specified in Section S.1.1. Figure S5 shows that the survival functions  $S(k \mid \mathbf{x}, \mathbf{z} = \mathbf{0})$  are similar to those in Figure 1 of the main paper, but with higher probabilities given to categories 1 and 5. In order to illustrate the effects of the linear terms  $\beta' \mathbf{z}$ , with  $\beta = (0.3, -0.5, 0.1)$ , Figure S7 shows the survival functions resulting from  $\lambda_1, \dots, \lambda_5$  being linear and  $z_2$  being equal to the 5%, 50% and 95% quantile of the underlying sampling distribution,  $z_2 \sim \text{Normal}(0, 1)$ , and  $z_1 = z_3 = 0$ . We see that this leads to moderate changes in the probabilities, in particular, for categories 1 and 5.

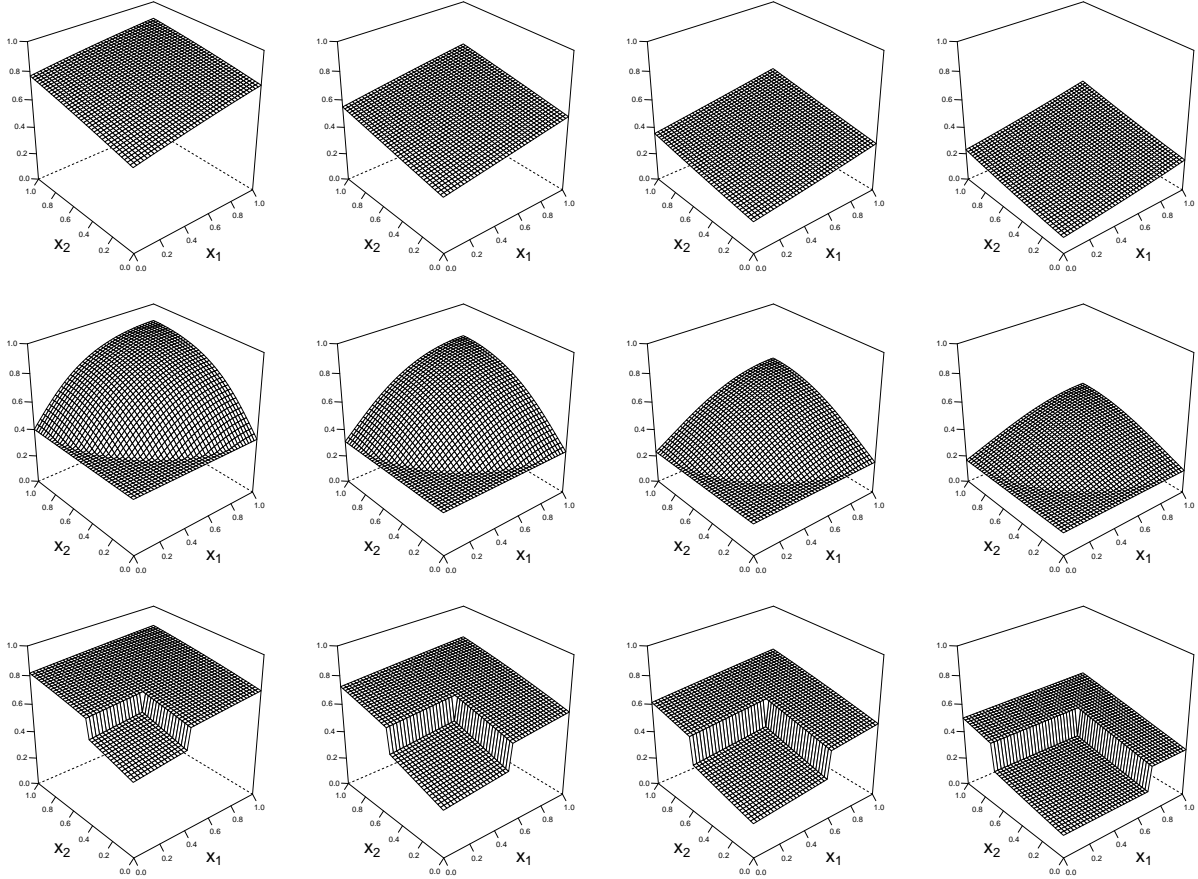

Figure S5: Graphical displays of the survival functions  $S(2 \mid \cdot), \dots, S(5 \mid \cdot)$  (left to right) for  $\mathbf{z} = \mathbf{0}$  considered in Section 3.2: linear functions (top), continuous (middle), and discontinuous (bottom).

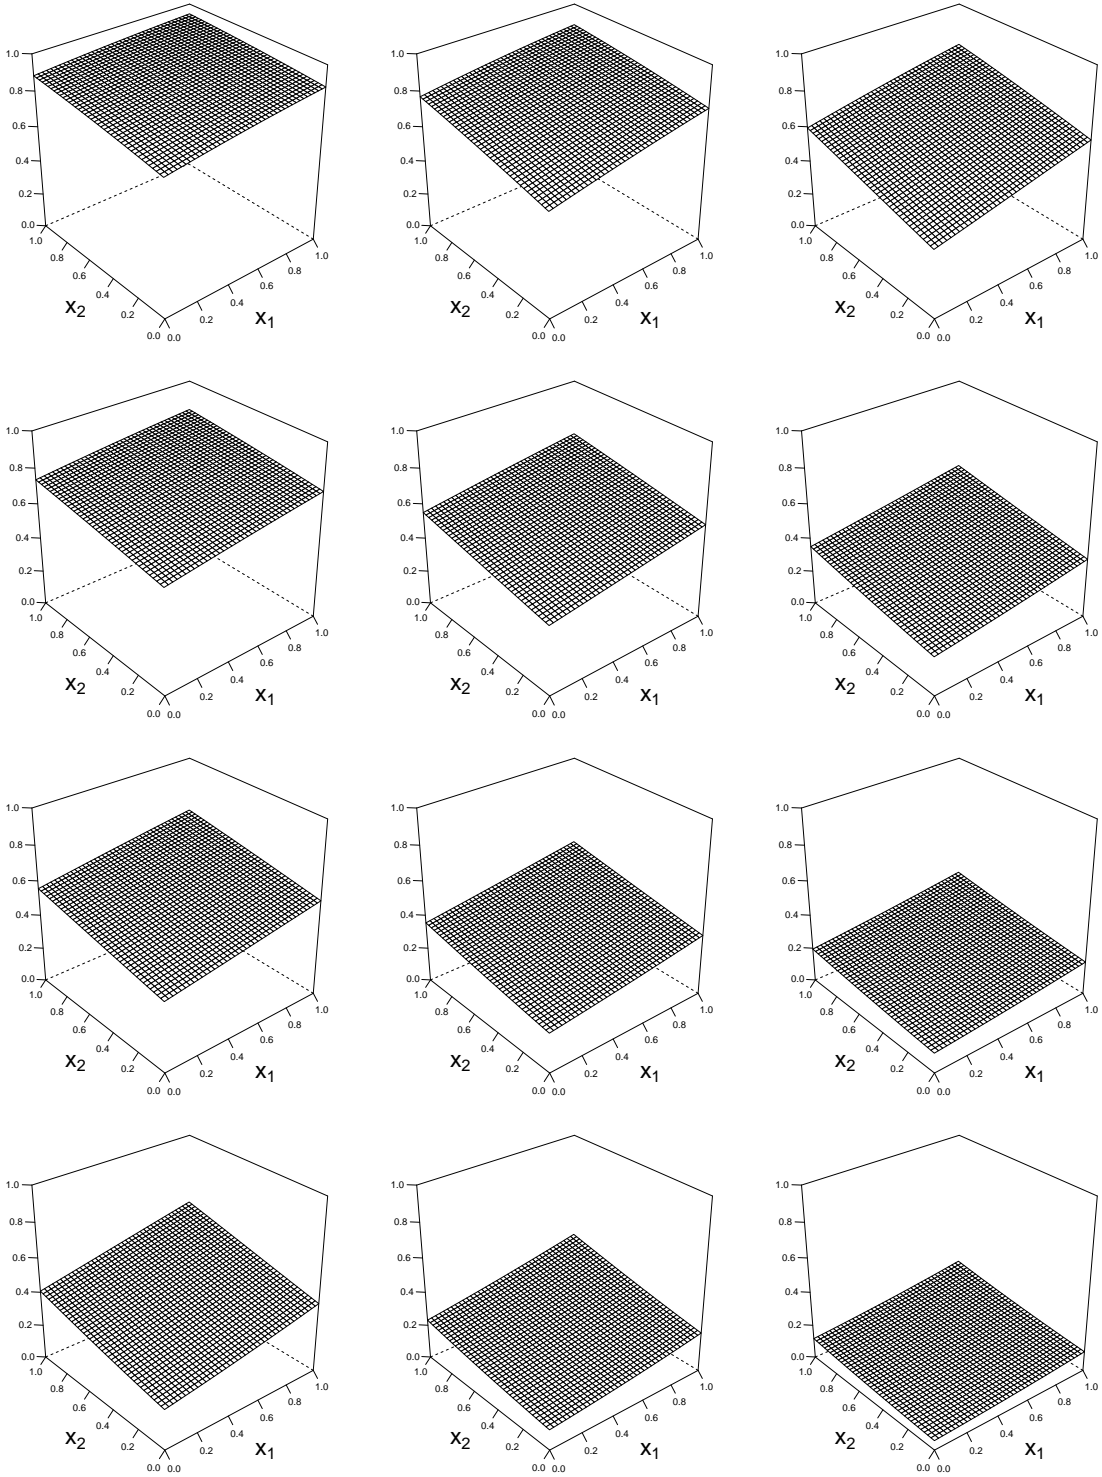

Figure S6: Graphical displays of the survival functions  $S(2 | \cdot), \dots, S(5 | \cdot)$  (top to bottom) for the linear functions  $\lambda_1, \dots, \lambda_5$  considered in Section 3.2. From left to right, the values for  $\mathbf{z}$  are  $\mathbf{z} = (0, -1.96, 0)$ ,  $\mathbf{z} = (0, 0, 0)$  and  $\mathbf{z} = (0, 1.96, 0)$ .

## S2.2 Posterior estimates for regression coefficients $\beta_1$ , $\beta_2$ and $\beta_3$

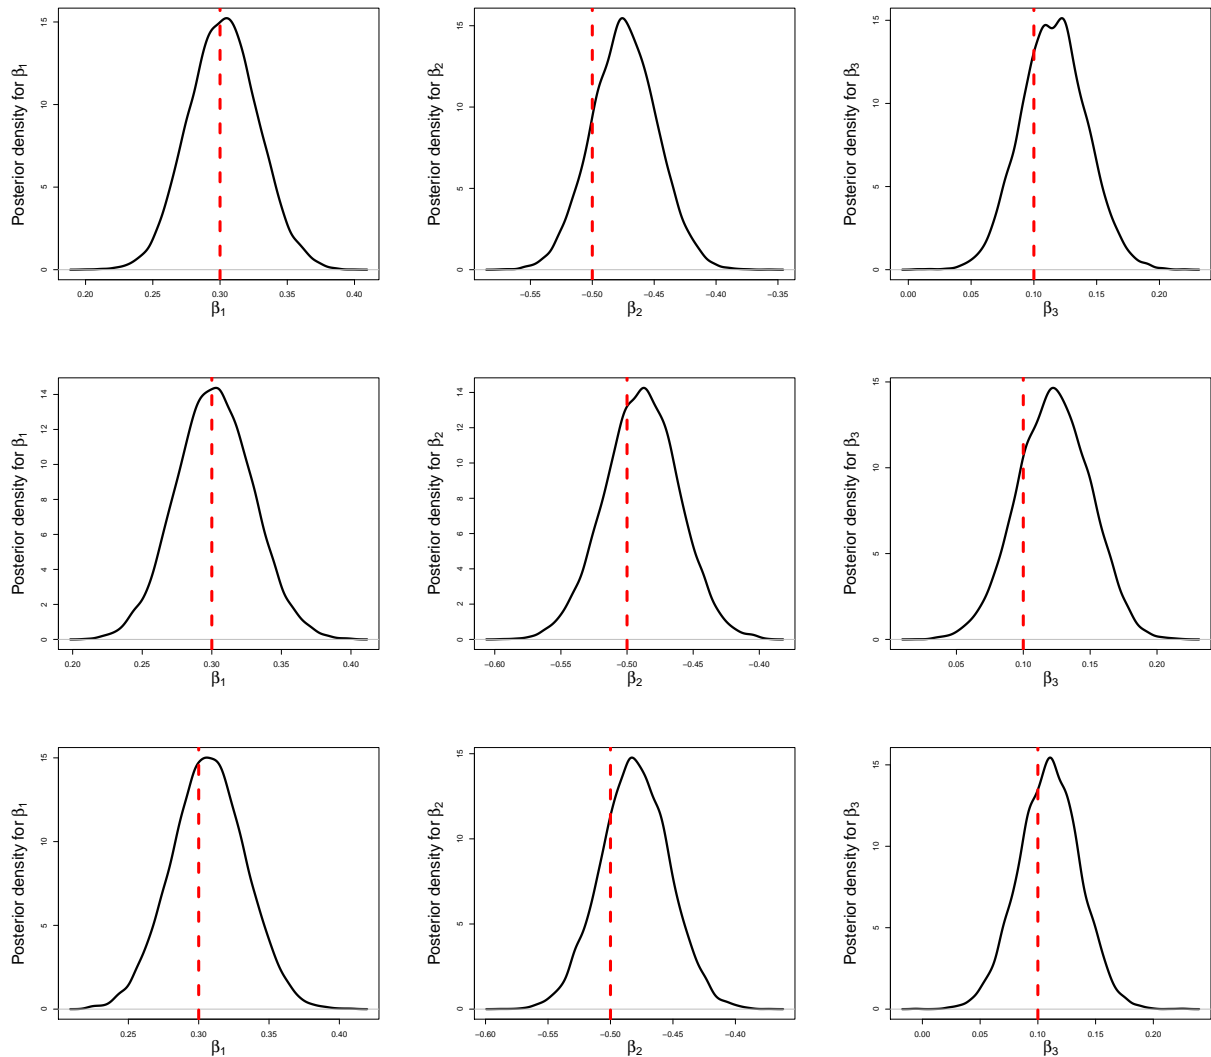

Figure S7: Posterior density estimates for  $\beta_1, \beta_2$  and  $\beta_3$  (left to right) for the simulations in Section 3.2. From top to bottom, the estimates correspond to the linear, continuous and discontinuous survival functions. The dashed lines correspond to the true values.

### S2.3 Model performance

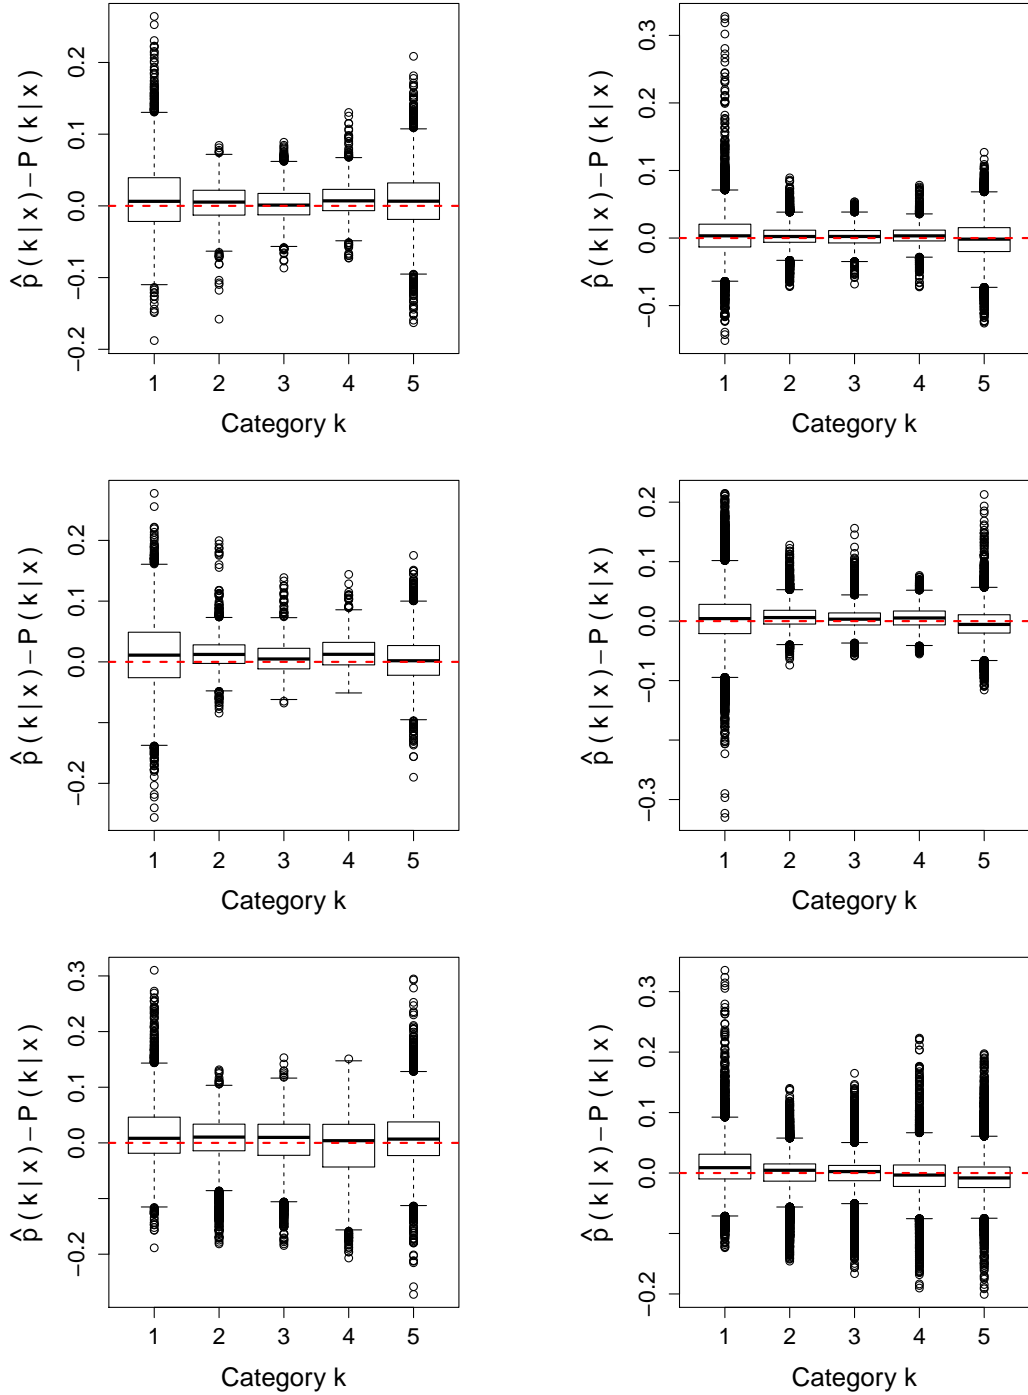

Figure S8: Boxplots of the difference  $\hat{p}(Y = y_n | \mathbf{x}_n) - \mathbb{P}(Y = y_n | \mathbf{x}_n)$  between the estimated and true probabilities for the  $K = 5$  categories across 20 simulated data sets with  $N = 1000$  (left) and  $N = 5000$  (right) data points. From top to bottom, the estimates correspond to the linear, continuous and discontinuous survival functions.

## S3 Supplementary Material for Section 4

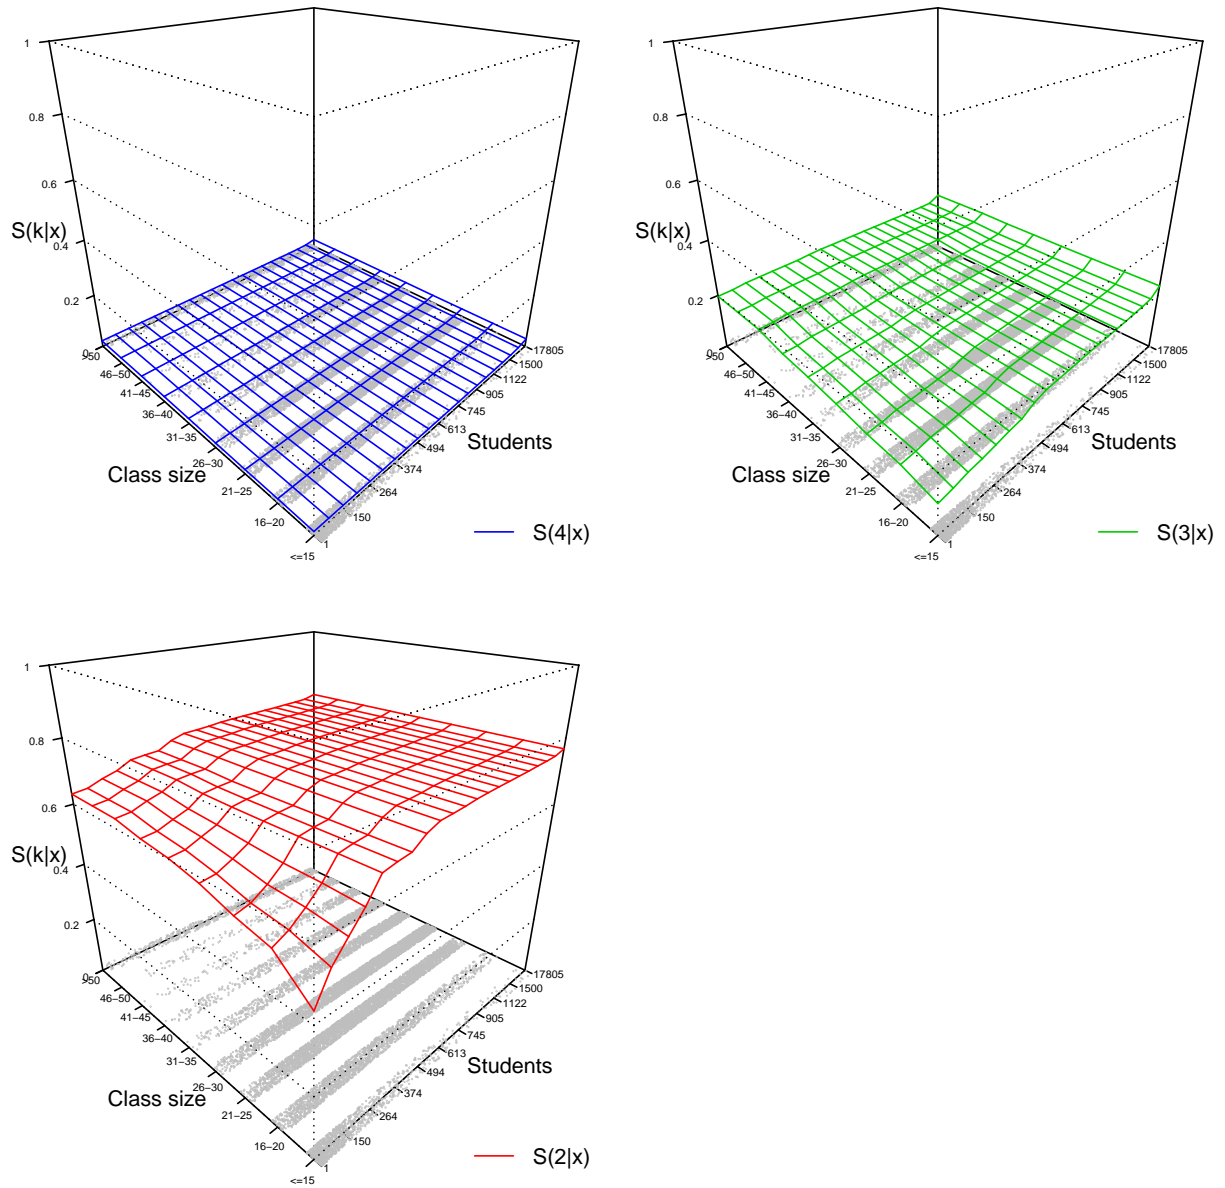

Figure S9: A perspective plot of the posterior mean regression surfaces for the three cumulative response category probabilities in the PISA data analysis. The jittered dots show the covariate coordinates of the data points.

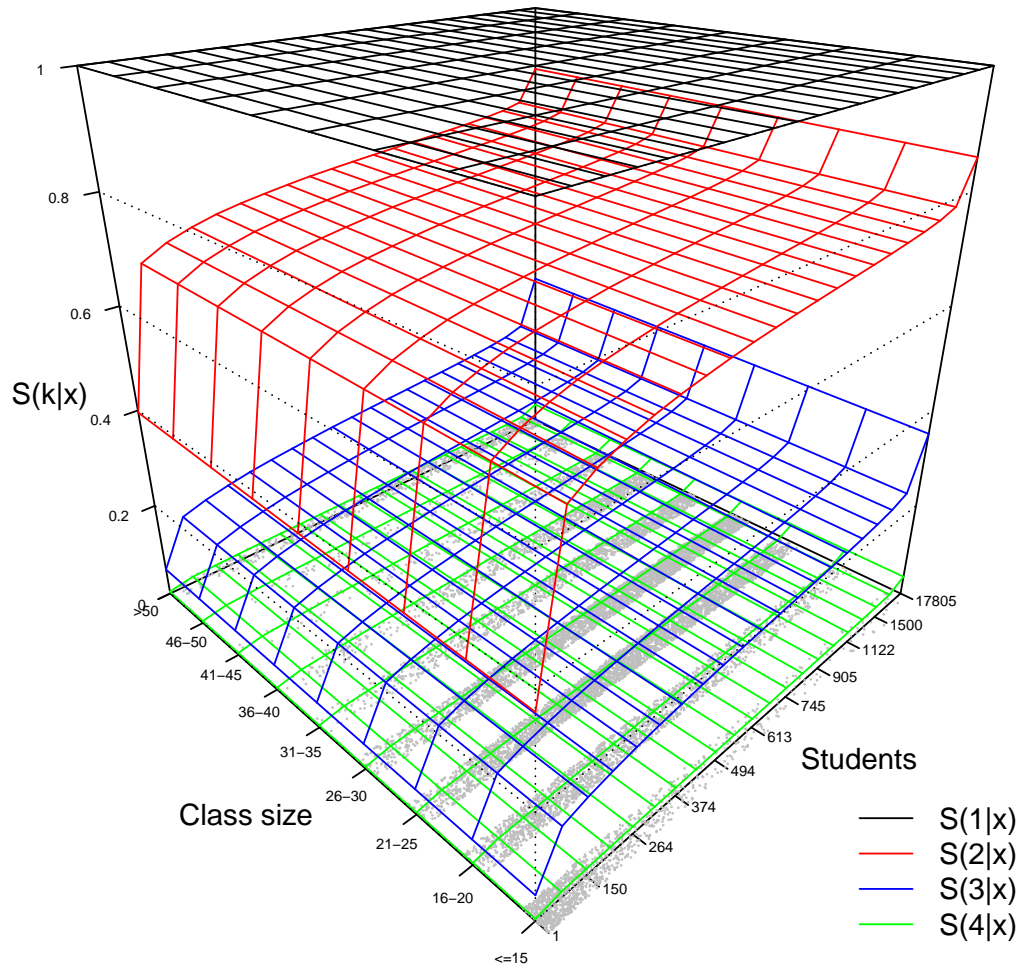

Figure S10: A perspective plot of the posterior mean regression surfaces for the three cumulative response category probabilities under the proportional odds model for PISA data. The jittered dots show the covariate coordinates of the data points.

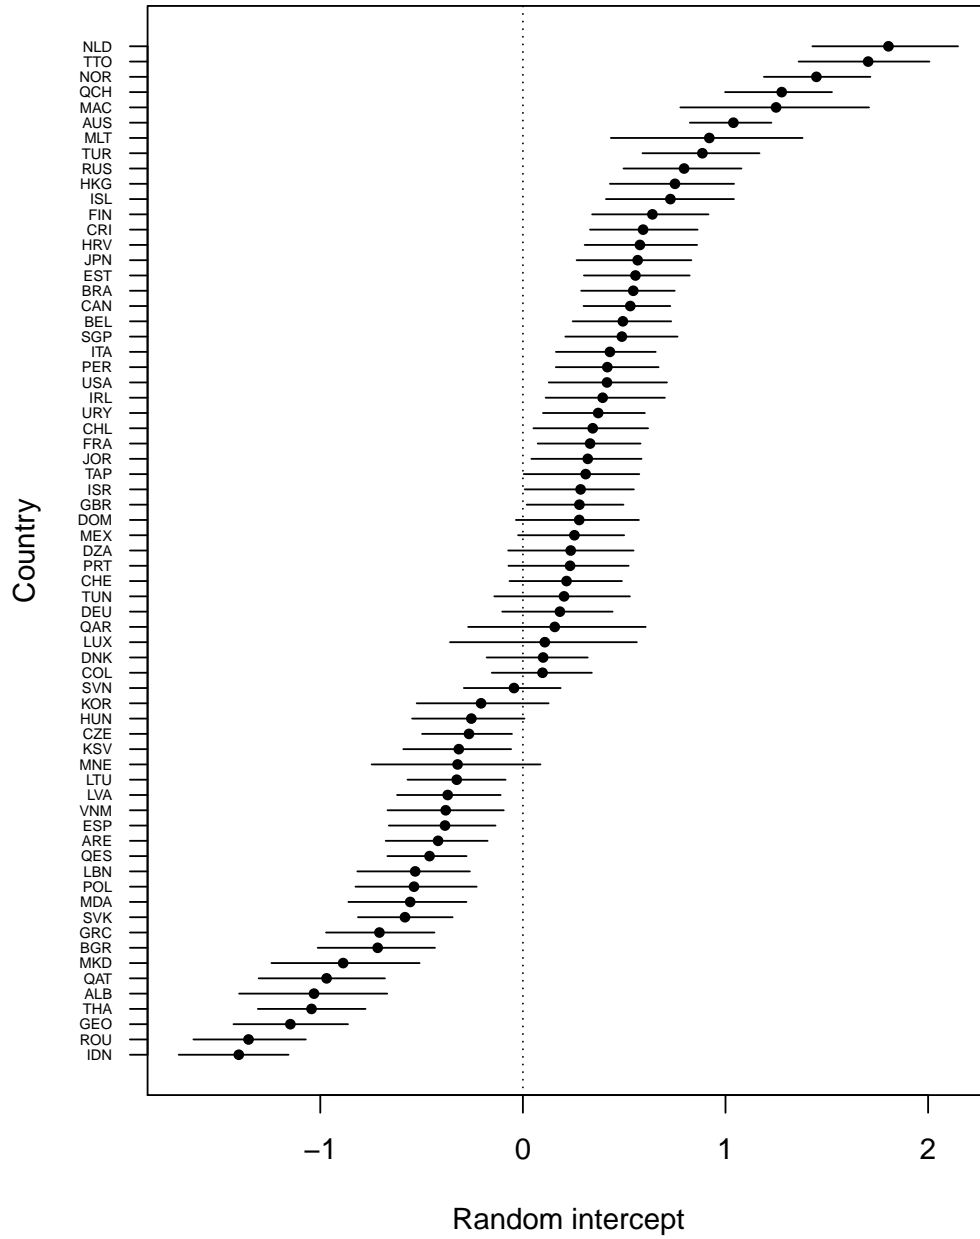

Figure S11: Posterior means and 90% credible intervals for the country-specific random intercept terms in the model for PISA data.

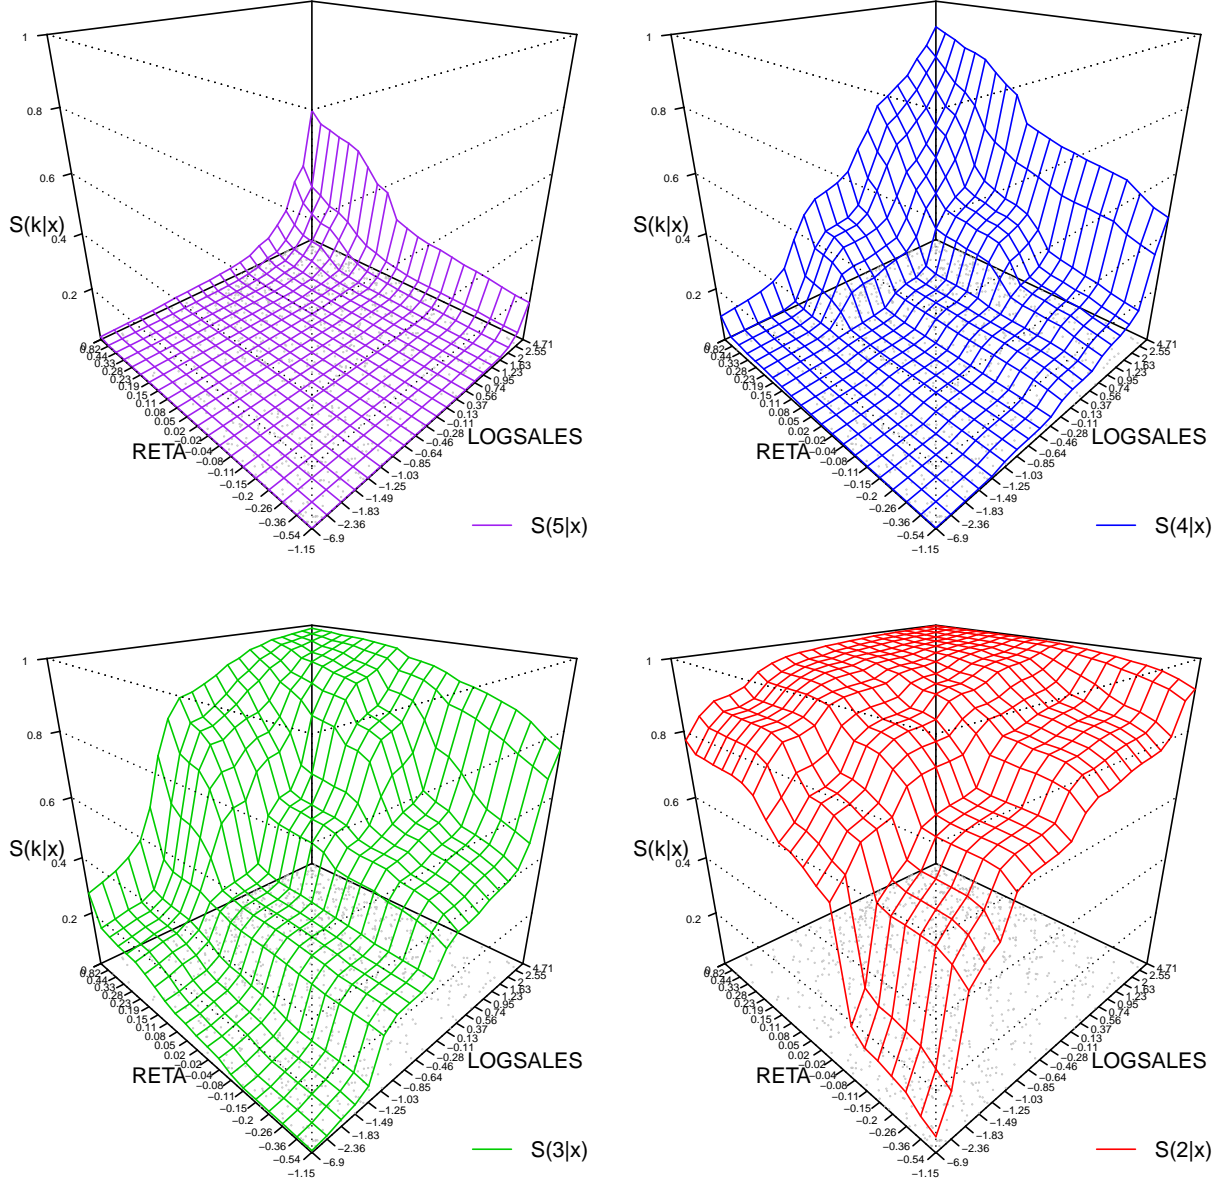

Figure S12: A perspective plot of standardized posterior mean regression surfaces for the four cumulative response category probabilities as functions of covariates RETA and LOGSALES in the credit score data. The dots show the covariate coordinates of the data points.
